# Supplementary material for: Long-Term Memory-Guided Enhancement for Target Perception in Audio-Language Models
Source: arXiv:2609.36577 source file (2026-09-29)
Supplement: Supplementary file 1 [file App_A.tex]

\appendix

\section{Detailed Twenty-Class Results}
\label{app:detailed_results}

This appendix reports the complete class-wise results of Qwen2-Audio, Kimi-Audio, and Step-Audio-2-mini under constrained classification, free-form classification, and prompt-free retrieval.
\subsection{Qwen2-Audio}

\begin{table}[H]
\centering
\caption{Class-wise constrained-classification accuracy (\%) of Qwen2-Audio.}
\label{tab:qwen_constrained_classwise}
\scriptsize
\setlength{\tabcolsep}{3pt}
\resizebox{\columnwidth}{!}{%
\begin{tabular}{lccccc}
\hline
Class & Clean & Mixed & PCA ($N=20$) & PCA ($N=50$) & PCA ($N=100$) \\
\hline
Piano             & 85 & 0  & 38  & 49  & 44  \\
Dog vocalization  & 86 & 14 & 100 & 100 & 99  \\
Human speech      & 94 & 64 & 100 & 100 & 100 \\
Flute             & 43 & 1  & 5   & 9   & 5   \\
Organ             & 61 & 1  & 38  & 50  & 35  \\
Classical guitar  & 87 & 3  & 63  & 77  & 64  \\
Violin            & 92 & 8  & 67  & 73  & 74  \\
Trumpet           & 64 & 3  & 63  & 11  & 17  \\
Clarinet          & 55 & 0  & 1   & 1   & 4   \\
Alto saxophone    & 24 & 3  & 0   & 10  & 0   \\
Drums             & 87 & 1  & 63  & 55  & 74  \\
Cat meow          & 100 & 40 & 100 & 100 & 100 \\
Cow moo           & 84 & 7  & 15  & 13  & 17  \\
Frog croak        & 0  & 0  & 0   & 0   & 0   \\
Crow call         & 29 & 1  & 0   & 0   & 0   \\
Glass breaking    & 88 & 12 & 100 & 100 & 100 \\
Car horn          & 77 & 7  & 27  & 61  & 78  \\
Baby crying       & 39 & 14 & 0   & 0   & 3   \\
Door slam         & 91 & 10 & 88  & 86  & 86  \\
Alarm             & 52 & 3  & 76  & 84  & 84  \\
\hline
Average           & 66.90 & 9.60 & 47.20 & 48.95 & 49.20 \\
\hline
\end{tabular}
}
\end{table}
\begin{table}[H]
\centering
\caption{Class-wise free-form classification accuracy (\%) of Qwen2-Audio.}
\label{tab:qwen_freeform_classwise}
\scriptsize
\setlength{\tabcolsep}{3pt}
\resizebox{\columnwidth}{!}{%
\begin{tabular}{lccccc}
\hline
Class & Clean & Mixed & PCA ($N=20$) & PCA ($N=50$) & PCA ($N=100$) \\
\hline
Piano             & 0  & 1  & 0   & 0   & 0   \\
Dog vocalization  & 83 & 31 & 100 & 100 & 100 \\
Human speech      & 3  & 0  & 0   & 0   & 0   \\
Flute             & 2  & 0  & 0   & 0   & 0   \\
Organ             & 38 & 0  & 0   & 0   & 0   \\
Classical guitar  & 5  & 1  & 1   & 0   & 0   \\
Violin            & 3  & 0  & 0   & 0   & 0   \\
Trumpet           & 15 & 0  & 0   & 0   & 0   \\
Clarinet          & 0  & 0  & 0   & 0   & 0   \\
Alto saxophone    & 2  & 1  & 0   & 0   & 0   \\
Drums             & 37 & 0  & 0   & 1   & 1   \\
Cat meow          & 89 & 20 & 95  & 91  & 89  \\
Cow moo           & 79 & 9  & 79  & 52  & 80  \\
Frog croak        & 0  & 0  & 0   & 0   & 0   \\
Crow call         & 38 & 4  & 0   & 0   & 0   \\
Glass breaking    & 72 & 4  & 50  & 82  & 85  \\
Car horn          & 83 & 16 & 100 & 100 & 100 \\
Baby crying       & 0  & 0  & 0   & 0   & 0   \\
Door slam         & 48 & 6  & 0   & 0   & 0   \\
Alarm             & 44 & 3  & 100 & 98  & 97  \\
\hline
Average           & 32.05 & 4.80 & 26.25 & 26.20 & 27.60 \\
\hline
\end{tabular}
}
\end{table}

\begin{table}[H]
\centering
\caption{Class-wise prompt-free retrieval accuracy (\%) of Qwen2-Audio.}
\label{tab:qwen_retrieval_classwise}
\scriptsize
\setlength{\tabcolsep}{3pt}
\resizebox{\columnwidth}{!}{%
\begin{tabular}{lccccc}
\hline
Class & Clean & Mixed & PCA ($N=20$) & PCA ($N=50$) & PCA ($N=100$) \\
\hline
Piano             & 99  & 5  & 100 & 100 & 100 \\
Dog vocalization  & 75  & 0  & 44  & 20  & 6   \\
Human speech      & 100 & 21 & 100 & 100 & 100 \\
Flute             & 76  & 0  & 100 & 100 & 100 \\
Organ             & 87  & 0  & 61  & 65  & 64  \\
Classical guitar  & 91  & 23 & 100 & 100 & 100 \\
Violin            & 95  & 0  & 82  & 83  & 87  \\
Trumpet           & 77  & 4  & 100 & 90  & 90  \\
Clarinet          & 88  & 3  & 13  & 16  & 26  \\
Alto saxophone    & 79  & 9  & 98  & 100 & 98  \\
Drums             & 93  & 8  & 100 & 100 & 100 \\
Cat meow          & 96  & 6  & 100 & 100 & 100 \\
Cow moo           & 97  & 6  & 100 & 100 & 100 \\
Frog croak        & 100 & 5  & 100 & 100 & 100 \\
Crow call         & 78  & 10 & 61  & 61  & 60  \\
Glass breaking    & 95  & 9  & 100 & 100 & 100 \\
Car horn          & 83  & 14 & 100 & 100 & 100 \\
Baby crying       & 86  & 24 & 100 & 100 & 100 \\
Door slam         & 92  & 9  & 100 & 100 & 100 \\
Alarm             & 71  & 9  & 76  & 100 & 91  \\
\hline
Average           & 87.90 & 8.25 & 86.75 & 86.75 & 86.10 \\
\hline
\end{tabular}
}
\end{table}
\subsection{Kimi-Audio}
\begin{table}[H]
\centering
\caption{Class-wise constrained-classification accuracy (\%) of Kimi-Audio.}
\label{tab:kimi_constrained_classwise}
\scriptsize
\setlength{\tabcolsep}{3pt}
\resizebox{\columnwidth}{!}{%
\begin{tabular}{lccccc}
\hline
Class & Clean & Mixed & PCA ($N=20$) & PCA ($N=50$) & PCA ($N=100$) \\
\hline
Piano             & 100 & 28 & 100 & 100 & 100 \\
Dog vocalization  & 90  & 14 & 100 & 91  & 84  \\
Human speech      & 84  & 10 & 29  & 29  & 26  \\
Flute             & 2   & 0  & 0   & 0   & 0   \\
Organ             & 13  & 4  & 5   & 10  & 11  \\
Classical guitar  & 91  & 4  & 96  & 98  & 99  \\
Violin            & 12  & 3  & 34  & 10  & 26  \\
Trumpet           & 45  & 0  & 49  & 35  & 20  \\
Clarinet          & 79  & 22 & 99  & 98  & 100 \\
Alto saxophone    & 1   & 3  & 0   & 0   & 0   \\
Drums             & 75  & 0  & 75  & 100 & 100 \\
Cat meow          & 66  & 16 & 60  & 65  & 68  \\
Cow moo           & 91  & 12 & 76  & 88  & 89  \\
Frog croak        & 0   & 0  & 0   & 0   & 0   \\
Crow call         & 45  & 5  & 84  & 77  & 75  \\
Glass breaking    & 95  & 9  & 100 & 100 & 99  \\
Car horn          & 72  & 6  & 88  & 94  & 92  \\
Baby crying       & 36  & 7  & 37  & 39  & 43  \\
Door slam         & 92  & 4  & 70  & 46  & 41  \\
Alarm             & 75  & 19 & 92  & 85  & 79  \\
\hline
Average           & 58.20 & 8.30 & 59.70 & 58.25 & 57.60 \\
\hline
\end{tabular}
}
\end{table}
\begin{table}[H]
\centering
\caption{Class-wise free-form classification accuracy (\%) of Kimi-Audio.}
\label{tab:kimi_freeform_classwise}
\scriptsize
\setlength{\tabcolsep}{3pt}
\resizebox{\columnwidth}{!}{%
\begin{tabular}{lccccc}
\hline
Class & Clean & Mixed & PCA ($N=20$) & PCA ($N=50$) & PCA ($N=100$) \\
\hline
Piano             & 46  & 0  & 90  & 92  & 85 \\
Dog vocalization  & 76  & 17 & 97  & 73  & 62 \\
Human speech      & 100 & 12 & 68  & 65  & 68 \\
Flute             & 1   & 0  & 0   & 0   & 0  \\
Organ             & 1   & 0  & 0   & 0   & 0  \\
Classical guitar  & 62  & 13 & 97  & 95  & 96 \\
Violin            & 18  & 1  & 17  & 5   & 20 \\
Trumpet           & 15  & 0  & 58  & 48  & 55 \\
Clarinet          & 0   & 0  & 0   & 0   & 0  \\
Alto saxophone    & 0   & 0  & 0   & 0   & 0  \\
Drums             & 78  & 4  & 82  & 100 & 99 \\
Cat meow          & 91  & 16 & 100 & 100 & 100 \\
Cow moo           & 12  & 0  & 17  & 19  & 20 \\
Frog croak        & 0   & 1  & 0   & 0   & 0  \\
Crow call         & 14  & 0  & 3   & 15  & 12 \\
Glass breaking    & 55  & 0  & 44  & 34  & 29 \\
Car horn          & 43  & 6  & 70  & 88  & 80 \\
Baby crying       & 40  & 18 & 47  & 43  & 44 \\
Door slam         & 82  & 7  & 77  & 74  & 60 \\
Alarm             & 35  & 3  & 49  & 34  & 36 \\
\hline
Average           & 38.45 & 4.90 & 45.80 & 44.25 & 43.30 \\
\hline
\end{tabular}
}
\end{table}
\begin{table}[H]
\centering
\caption{Class-wise prompt-free retrieval accuracy (\%) of Kimi-Audio.}
\label{tab:kimi_retrieval_classwise}
\scriptsize
\setlength{\tabcolsep}{3pt}
\resizebox{\columnwidth}{!}{%
\begin{tabular}{lccccc}
\hline
Class & Clean & Mixed & PCA ($N=20$) & PCA ($N=50$) & PCA ($N=100$) \\
\hline
Piano             & 96  & 3  & 100 & 100 & 99 \\
Dog vocalization  & 63  & 0  & 71  & 26  & 32 \\
Human speech      & 100 & 53 & 97  & 89  & 91 \\
Flute             & 35  & 0  & 3   & 2   & 2  \\
Organ             & 81  & 1  & 43  & 42  & 62 \\
Classical guitar  & 88  & 25 & 86  & 83  & 78 \\
Violin            & 70  & 12 & 71  & 79  & 79 \\
Trumpet           & 84  & 8  & 89  & 77  & 84 \\
Clarinet          & 83  & 0  & 79  & 88  & 80 \\
Alto saxophone    & 85  & 7  & 79  & 82  & 87 \\
Drums             & 94  & 2  & 88  & 85  & 85 \\
Cat meow          & 93  & 8  & 100 & 100 & 100 \\
Cow moo           & 98  & 27 & 98  & 98  & 98 \\
Frog croak        & 100 & 1  & 100 & 100 & 100 \\
Crow call         & 60  & 3  & 33  & 60  & 53 \\
Glass breaking    & 97  & 6  & 100 & 100 & 94 \\
Car horn          & 58  & 7  & 69  & 64  & 78 \\
Baby crying       & 88  & 42 & 91  & 87  & 84 \\
Door slam         & 84  & 8  & 71  & 74  & 75 \\
Alarm             & 51  & 12 & 44  & 16  & 25 \\
\hline
Average           & 80.40 & 11.25 & 75.60 & 72.60 & 74.30 \\
\hline
\end{tabular}
}
\end{table}
\subsection{Step-Audio-2-mini}

\begin{table}[H]
\centering
\caption{Class-wise constrained-classification accuracy (\%) of Step-Audio-2-mini.}
\label{tab:stepfun_constrained_classwise}
\scriptsize
\setlength{\tabcolsep}{3pt}
\resizebox{\columnwidth}{!}{%
\begin{tabular}{lccccc}
\hline
Class & Clean & Mixed & PCA ($N=20$) & PCA ($N=50$) & PCA ($N=100$) \\
\hline
Piano             & 100 & 0  & 29 & 58 & 69 \\
Dog vocalization  & 90  & 23 & 96 & 97 & 92 \\
Human speech      & 98  & 65 & 98 & 97 & 95 \\
Flute             & 32  & 4  & 0  & 0  & 1  \\
Organ             & 30  & 2  & 1  & 1  & 2  \\
Classical guitar  & 92  & 7  & 48 & 46 & 46 \\
Violin            & 96  & 6  & 57 & 64 & 67 \\
Trumpet           & 68  & 3  & 26 & 34 & 38 \\
Clarinet          & 90  & 5  & 15 & 30 & 33 \\
Alto saxophone    & 14  & 1  & 0  & 0  & 0  \\
Drums             & 90  & 2  & 48 & 31 & 43 \\
Cat meow          & 96  & 22 & 56 & 58 & 60 \\
Cow moo           & 91  & 8  & 80 & 80 & 86 \\
Frog croak        & 48  & 2  & 19 & 20 & 20 \\
Crow call         & 46  & 4  & 14 & 10 & 13 \\
Glass breaking    & 90  & 12 & 57 & 73 & 54 \\
Car horn          & 75  & 7  & 71 & 78 & 51 \\
Baby crying       & 41  & 16 & 27 & 28 & 37 \\
Door slam         & 92  & 10 & 45 & 76 & 48 \\
Alarm             & 71  & 6  & 54 & 35 & 41 \\
\hline
Average           & 72.50 & 10.25 & 42.05 & 45.80 & 44.80 \\
\hline
\end{tabular}
}
\end{table}
\begin{table}[H]
\centering
\caption{Class-wise free-form classification accuracy (\%) of Step-Audio-2-mini.}
\label{tab:stepfun_freeform_classwise}
\scriptsize
\setlength{\tabcolsep}{3pt}
\resizebox{\columnwidth}{!}{%
\begin{tabular}{lccccc}
\hline
Class & Clean & Mixed & PCA ($N=20$) & PCA ($N=50$) & PCA ($N=100$) \\
\hline
Piano             & 78 & 2  & 54 & 49 & 29 \\
Dog vocalization  & 80 & 26 & 87 & 92 & 89 \\
Human speech      & 80 & 19 & 55 & 63 & 62 \\
Flute             & 22 & 0  & 1  & 1  & 8  \\
Organ             & 2  & 0  & 0  & 0  & 0  \\
Classical guitar  & 66 & 10 & 44 & 37 & 30 \\
Violin            & 81 & 4  & 62 & 75 & 79 \\
Trumpet           & 52 & 1  & 13 & 20 & 32 \\
Clarinet          & 71 & 3  & 25 & 28 & 35 \\
Alto saxophone    & 31 & 6  & 2  & 2  & 6  \\
Drums             & 65 & 4  & 88 & 74 & 79 \\
Cat meow          & 98 & 24 & 84 & 86 & 87 \\
Cow moo           & 79 & 3  & 65 & 66 & 71 \\
Frog croak        & 0  & 1  & 0  & 0  & 0  \\
Crow call         & 29 & 0  & 10 & 8  & 10 \\
Glass breaking    & 80 & 1  & 40 & 54 & 33 \\
Car horn          & 80 & 7  & 66 & 58 & 65 \\
Baby crying       & 29 & 13 & 39 & 34 & 51 \\
Door slam         & 83 & 14 & 76 & 92 & 90 \\
Alarm             & 40 & 5  & 38 & 20 & 37 \\
\hline
Average           & 57.30 & 7.15 & 42.45 & 42.95 & 44.65 \\
\hline
\end{tabular}
}
\end{table}
\begin{table}[H]
\centering
\caption{Class-wise prompt-free retrieval accuracy (\%) of Step-Audio-2-mini.}
\label{tab:stepfun_retrieval_classwise}
\scriptsize
\setlength{\tabcolsep}{3pt}
\resizebox{\columnwidth}{!}{%
\begin{tabular}{lccccc}
\hline
Class & Clean & Mixed & PCA ($N=20$) & PCA ($N=50$) & PCA ($N=100$) \\
\hline
Piano             & 99  & 2  & 100 & 100 & 100 \\
Dog vocalization  & 74  & 0  & 1   & 0   & 0   \\
Human speech      & 100 & 60 & 100 & 100 & 100 \\
Flute             & 72  & 0  & 50  & 51  & 72  \\
Organ             & 87  & 0  & 32  & 41  & 53  \\
Classical guitar  & 89  & 32 & 61  & 100 & 100 \\
Violin            & 94  & 0  & 100 & 91  & 83  \\
Trumpet           & 81  & 1  & 91  & 85  & 91  \\
Clarinet          & 90  & 2  & 26  & 37  & 64  \\
Alto saxophone    & 82  & 13 & 99  & 100 & 100 \\
Drums             & 93  & 5  & 100 & 100 & 100 \\
Cat meow          & 99  & 7  & 100 & 100 & 100 \\
Cow moo           & 98  & 10 & 100 & 100 & 100 \\
Frog croak        & 100 & 3  & 100 & 100 & 100 \\
Crow call         & 81  & 9  & 94  & 94  & 89  \\
Glass breaking    & 98  & 7  & 56  & 100 & 60  \\
Car horn          & 86  & 10 & 100 & 100 & 100 \\
Baby crying       & 88  & 31 & 99  & 97  & 96  \\
Door slam         & 91  & 9  & 100 & 100 & 97  \\
Alarm             & 77  & 8  & 61  & 77  & 45  \\
\hline
Average           & 88.95 & 10.45 & 78.50 & 83.65 & 82.50 \\
\hline
\end{tabular}
}
\end{table}
